# Supplementary material for: An Energy-Based Interface Detection Method for Phase Change Processes in Nanoconfinements
Source: arXiv:2106.02238 ancillary file (2021-06-04)
Supplement: Supplementary file 1 [file Supporting_Information.pdf]

Supporting Information for

# An Energy-Based Interface Detection Method for Phase Change Processes in Nanoconfinements

Mustafa Ozsipahi[a], Yigit Akkus[b], Chinh Thanh Nguyen[a] Ali Beskok[a]

[a]Southern Methodist University, Dallas, Texas 75205, USA
[b]ASELSAN Inc., Ankara 06200, Turkey

1. Molecular Dynamics Simulation Details
2. Surface Tension Calculations

## 1. Molecular Dynamics Simulation Details

Three different simulation models were constructed to investigate various interface detection methods. Domain sizes of $(L \times H \times W)$ $62.720 \times 9.016 \times 3.724\,\mathrm{nm}^3$, $31.360 \times 5.096 \times 3.724\,\mathrm{nm}^3$, and $15.680 \times 3.136 \times 3.724\,\mathrm{nm}^3$ were selected for Model 1 (M1), Model 2 (M2), and Model 3 (M3), respectively. All models were geometrically scaled, while the depth (3.724 nm) and thickness (0.588 nm) of the solid walls were kept constant. Periodic boundary conditions were applied in all three directions. Platinum (Pt) and Argon (Ar) were used in simulations due to their well-known interaction potentials. The channel walls were modeled using Pt atoms composed of 4 solid layers modeled with (1,0,0) plane facing the fluid. The outermost layer of the walls were fixed at their lattice positions. The embedded-atom method (EAM) was used for the interatomic forces of Pt atoms [1]. Lennard–Jones (L-J) 12-6 potential was used to model van der Waals interactions between Ar-Pt and Ar-Ar atoms. The interaction parameters were $\sigma_{\mathrm{Ar}}$=0.34 nm, $\sigma_{\mathrm{Ar-Pt}}$=0.3085 nm, $\epsilon_{\mathrm{Ar}}$=0.01042 eV, and $\epsilon_{\mathrm{Ar-Pt}}$=0.00558 eV [2]. The L-J potential was truncated at $3\sigma_{\mathrm{Ar}}$ to reduce the computational time [3]. The computational domain was divided into $\frac{\sigma}{7} \times \frac{\sigma}{7}$ rectangular prism bins to resolve the near-wall region. Simulations used 5 fs time steps.

Simulations started using the Maxwell-Boltzmann velocity distribution for liquid molecules at 110 K. The system was relaxed isothermally for 10 ns to reach an isothermal state using the Nosé–Hoover thermostat. Then microcanonical ensemble (NVE) (*i.e.*, constant number of atoms N, volume V, and energy E) was applied on Ar atoms for another 10 ns while keeping the solid atoms at 110 K using the thermostat. Two stable menisci were visible at the channel tips at the end of this stage. The density, KE, and PE were averaged using 400k samples between 12 to 20 ns. In the NEMD stage, equal heating and cooling (H/C) were applied at the channel ends corresponding to $1/8^{th}$ of the total channel length (on each side). During H/C, Ar atoms were kept in a microcanonical ensemble, and the system was simulated for 30 ns. Time averaging from 30 to 50 ns was obtained using 1M samples to minimize the statistical fluctuations in density, KE, PE and other variables.

The number of atoms used in various models were as follows: 16,575 Ar-12,800 Pt (M1), 4,200 Ar-6,400 Pt (M2), 1,035 Ar-3,280 Pt (M3). These numbers were carefully selected to match the thermodynamic state of Ar between each model for equilibrium simulations. Adding Ar atoms to the system changes the quality factor and radius of curvature (ROC). All three models yielded pinned-menisci at the channel tips under equilibrium MD simulations, as shown in Figs 1, 2 and 5 in the manuscript, while a stable menisci at the evaporator and a nearly flat interface at the condenser regions were observed during NEMD simulations (Fig. S1).

We additionally performed simulations with $3\epsilon_{\mathrm{Ar-Pt}}$ and $5\epsilon_{\mathrm{Ar-Pt}}$ to investigate the effects of increased wall attraction in the M2 case. The effect of fluid-wall interaction potential on the density and energy distributions near an interface are shown in Fig. S2. Increasing $\epsilon_{\mathrm{Ar-Pt}}$

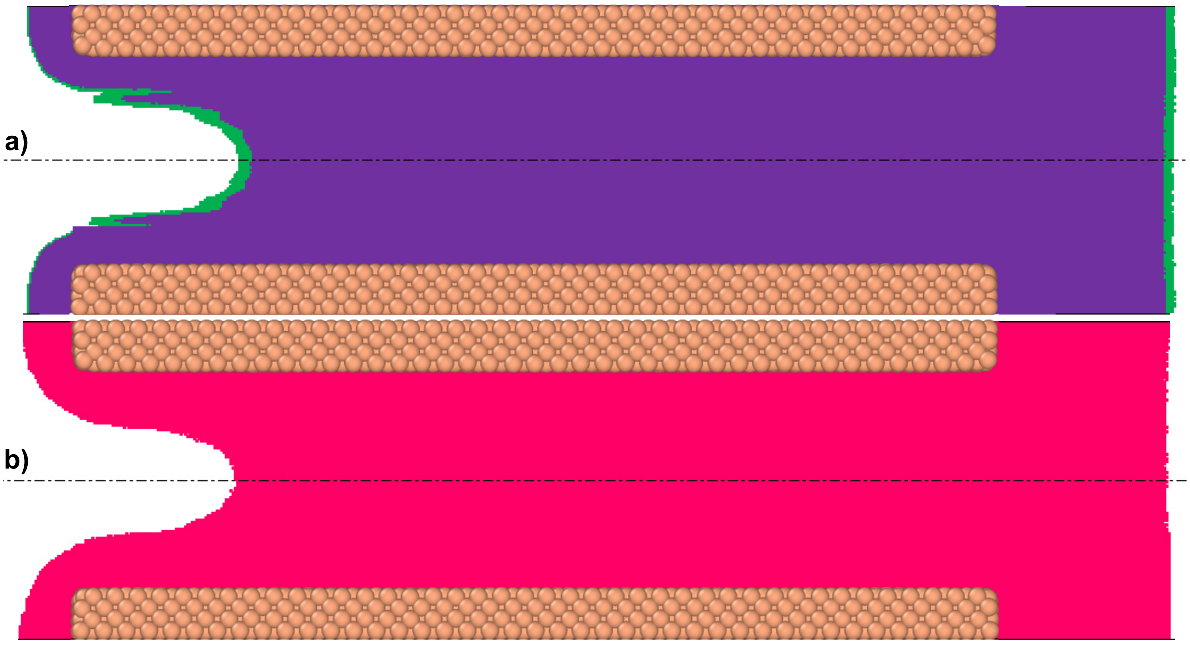


Figure S1: Liquid phase for the M2 case under 8 nW H/C and $3\epsilon_{\mathrm{Ar-Pt}}$ with **a)** density-based, and **b)** energy-based interface detection methods. The condenser section has mostly flat interface (right side) while the evaporator section (left side) shows a stable receded interface.

results in higher potential energy, and a thicker adsorbed layer. It is shown that energy-based surface detection can successfully predict the interface for various $\epsilon_{\mathrm{Ar-Pt}}$ values.

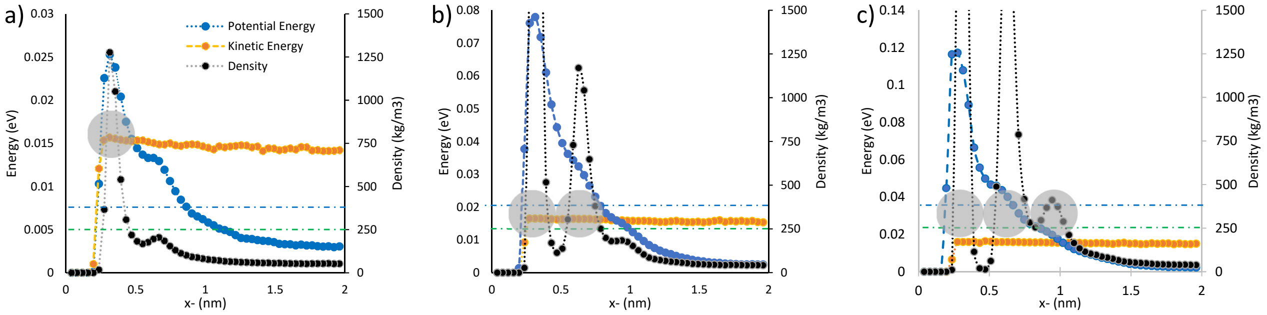


Figure S2: Near-wall region energy and density distributions for the M2 case under 8 nW H/C are shown for $\epsilon_{\mathrm{Ar-Pt}}$ values equaling to **a)** 0.0055, **b)** 0.0165, and **c)** 0.0275 eV . Molecular diameters are shown in the figure to indicate the scale, and green and blue dashed-dotted lines represent the density cutoff values of 250 and 350 $\mathrm{kg/m^3}$, respectively. Increasing $\epsilon_{\mathrm{Ar-Pt}}$ results in multiple near wall density peaks and this creates oscillations for the density based interface detection. However the energy based interface method naturally adopts to the density layering.

## 2. Surface Tension Calculations

Two different methods are used to calculate the liquid-vapor surface tension. First, the Young-Laplace equation states,

$$\Delta P = \frac{\gamma}{R}, \tag{S1}$$

where $\gamma$ is the liquid/vapor surface tension, $\Delta P$ is the pressure difference between the bulk liquid and vapor, and $R$ is the ROC of the meniscus. In order to calculate the surface tension, we need to compute $\Delta P$ and $R$. Components of the local stress tensor are calculated using the Irving-Kirkwood method [4], and the pressure is calculated by averaging the diagonal components of the stress tensor in the Cartesian coordinate system as follows:

$$P = \frac{S_{xx} + S_{yy} + S_{zz}}{3}. \tag{S2}$$

Since the liquid pressure inside the nanochannel fluctuates even at the channel center for the M2 case, selection of the calculation zone/slab (a group of bins) is important to find the pressure difference and surface tension. The influence of the slab thickness on the calculation of liquid-vapor interfacial tension was previously reported in [5]. Thus, six different slab sizes varying between 0.4 to 1.4 nm are selected and the corresponding liquid-vapor pressure differences are calculated.

Using NVE ensemble fixes the fluid density and energy in the system. Since there is no flow or heat flux, fixed energy simulations result in constant temperature. Therefore, the radius of curvature (ROC) is calculated using the equilibrium meniscus profiles. Since the meniscus is pinned at the channel tips, circular fits for ROC were applied near the center of the meniscus, nearly $3\sigma_{Ar}$ distance from each wall to avoid the wall effects in pressure and surface tension calculations. Two different curve fitting methods were applied in order to obtain ROC [6, 7]. These radii are used to predict the surface tension using Eqn. (S1).

In addition to the Young-Laplace equation, the liquid-vapor surface tension was calculated using MD data as follows:

$$\gamma = \int [S_N(x) - S_T(x)]dx, \tag{S3}$$

where $S_N$ and $S_T$ are the normal stress components, respectively. Specifically along the channel axis, $S_N = S_{xx}$ and $S_T = 0.5(S_{yy} + S_{zz})$; and $S_{xx}$, $S_{yy}$, and $S_{zz}$ are the three normal stress components in $x$, $y$, and $z$ directions, respectively. Contributions to Eqn. (S3) vanishes, when all normal stress components within a bin are equal. Isotropic normal stresses result in "pressure" as shown in Eqn. (S2). Whereas in the interface region, the corresponding calculation yields a finite liquid-vapor surface tension value. Figure S3 shows the spatial variation of the

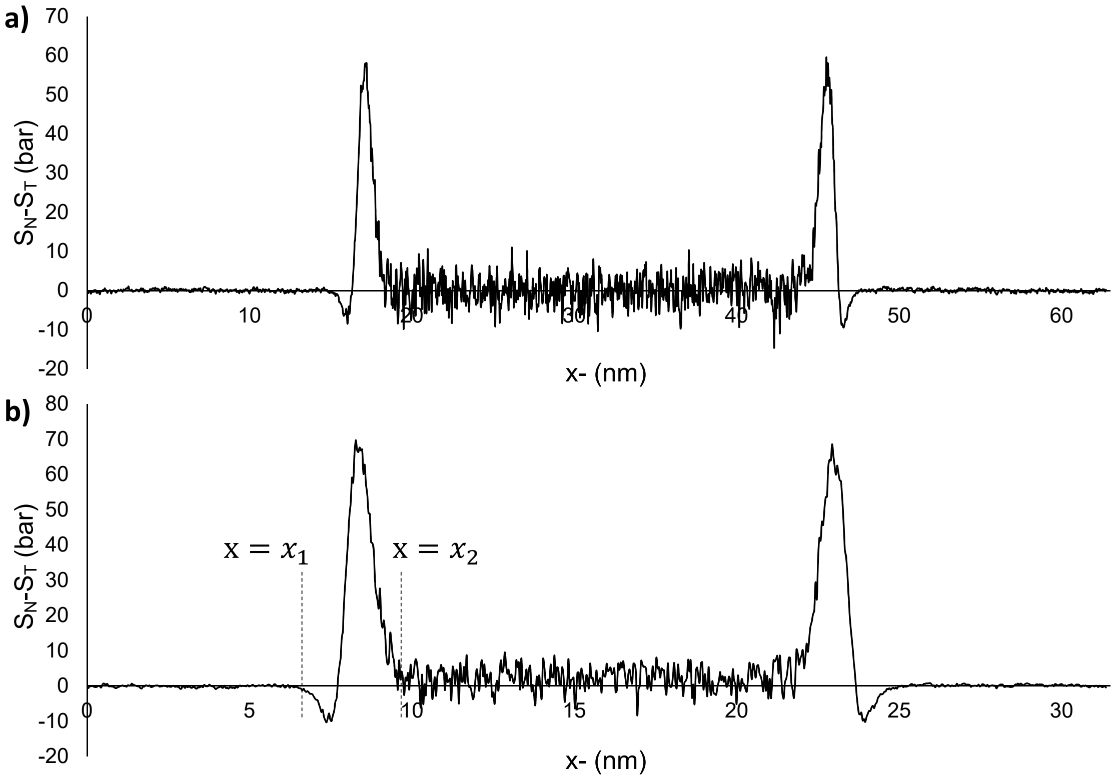


Figure S3: Variation of $S_N(x) - S_T(x)$ in axial direction of the channel for the **a)** M1 and **b)** M2 cases. Surface tension values are calculated by integration of this using Eqn. (S3).

integrant in Eqn. (S3) along the domain center, used for calculating $\gamma$ for the M1 and M2 cases. When the channel domain is large and the wall effects are sufficiently away from the channel center, such as in the M1 case, the integral in Eqn. (S3) can be taken along half of the entire computational domain However for the smaller M2 case, nanoconfinement causes density and pressure fluctuations even in the channel center, thus the integral to calculate the surface tension was taken from $x = x_1$ to $x = x_2$, which is the range of the liquid-vapor interface. This method of calculating the surface tension has been widely used in the literature before [8, 9]. In the manuscript, we compared the consistency of determining the ROC form various interface detection methods and MD calculated surface tension values, and have shown the superiority of the new energy based interface detection method while using the Young-Laplace equation.

# References

[1] S. M. Foiles, M. I. Baskes, and M. S. Daw. Embedded-atom-method functions for the FCC metals Cu, Ag, Au, Ni, Pd, Pt, and their alloys. *Phys. Rev. B*, 33(12):7983, 1986.

[2] S. Maruyama and T. Kimura. A study on thermal resistance over a solid-liquid interface by the molecular dynamics method. *Therm. Sci. Eng.*, 7(1):63–68, 1999.

[3] M. P. Allen and D. J. Tildesley. *Computer Simulation of Liquids.* Oxford: Clarendon Pr, 1987.

[4] J. H. Irving and J. G. Kirkwood. The statistical mechanical theory of transport processes. iv. the equations of hydrodynamics. *J. Chem. Phys.*, 18(6):817–829, 1950.

[5] S. Werth, S. V. Lishchuk, M. Horsch, and H. Hasse. The influence of the liquid slab thickness on the planar vapor–liquid interfacial tension. *Physica A*, 392(10):2359–2367, 2013.

[6] V. Pratt. Direct least-squares fitting of algebraic surfaces. *ACM SIGGRAPH computer graphics*, 21(4):145–152, 1987.

[7] I. Bucher. Circle fit, matlab central file exchange. retrieved april 28, 2021. `https://www.mathworks.com/matlabcentral/fileexchange/5557-circle-fit`, 2021.

[8] F. Biscay, A. Ghoufi, V. Lachet, and P. Malfreyt. Prediction of the surface tension of the liquid-vapor interface of alcohols from monte carlo simulations. *J. Phys. Chem. C*, 115(17):8670–8683, 2011.

[9] S. Yesudasan and S. C. Maroo. Origin of surface-driven passive liquid flows. *Langmuir*, 32(34):8593–8597, 2016.
